# Supplementary material for: Conformal Mirror Descent with Logarithmic Divergences
Source: arXiv:2209.02938 source file (2022-09-07)
Supplement: Supplementary file 1 [file supplement.tex]

\newpage
\appendix
\begin{appendices}

\section{Convergence analysis of conformal mirror descent in discrete time}%
\label{sec:convergence_analysis}

We prove the convergence of the \Acrlong{CBD} update in~\eqref{eq:feuler-tcmf}
under suitable assumptions on the objective $f$, for a given  $c_\lambda$-convex
$\varphi$ inducing the \Acrshort{CBD} using the \emph{convex} generator
$\Phi(\p)\defeq \frac{1}{\lambda}\left( e^{\lambda\varphi(\p)} -1 \right)$.
Before we can demonstrate a Lyapunov function for this algorithm, we need
a generalization of the relative \emph{smoothness} condition \cite{wilson18}.
A function $f$ is  $L$-smooth \wrt{} a strictly convex function $\phi$ if and
only if
\begin{equation*}
  \BD[f]{x}{y} \le  L\BD[\phi]{x}{y},\quad \forall
  (x,y)\in\dom(\phi)\cap\dom(f).
\end{equation*}
Generalizing this for our analysis of the induced $\lambda$-geometry, a function
$f$ is \emph{conformal} $L$-smooth \wrt{} a $c_\lambda$-convex function
$\varphi$ if and only if
\begin{equation} \label{eq:conformal_smooth}
  \BD[f]{x}{y} \le Le^{-\lambda\varphi(y)}\BD[\Phi]{x}{y} = Le^{\lambda\left(
  \varphi(x)-\varphi(y) \right) }\left( 1 - e^{-\lambda\LD{x}{y}} \right)
\end{equation}
Note that we recover the regular smoothness condition when $\lambda = 0$ or when
$\varphi(x) < 0 \ \forall x\in\dom(\varphi)$. When $\varphi(x) > 0$ however, the
conformal smoothness corresponds to a stricter assumption due to the conformal
factor tightening the upper bound in~\eqref{eq:conformal_smooth}.
To prove a convergence rate for the \acrshort{CBD} iterates, we first prove the
existence of a Lyapunov potential (the discrete analogue
of~\eqref{eqn:Lyapunov.candidate}).
\begin{theorem}[Lyapunov potential for the \acrshort{CBD}]
  Let $f$ be convex in  $\p$. Then the function
  \begin{equation}\label{eq:lyapunov_discrete}
    E_k \defeq \BD[\Phi]{\p^*}{\p_k}
    + \delta\sum_{s=1}^{k}e^{\lambda\varphi(\p_{s-1})}(f(\p_s) - f(\p^*));\quad
    k\ge 1
  \end{equation}
  satsifies $E_{k+1} \le E_k \ \forall k\ge 1$, where $\Phi \defeq
  \frac{1}{\lambda}\left( e^{\lambda\varphi} -1 \right)$.
\end{theorem}
\begin{proof}
  With $\Phi \defeq \frac{1}{\lambda}\left( e^{\lambda\varphi}-1 \right)$, the
  difference can checked as
  \begin{equation*}
    \begin{split}
      \frac{E_{k+1}-E_k}{\delta} &= \overbrace{\frac{1}{\delta}\left(\Phi(\p_k)
      + \DP{\grad\Phi(\p_k)}{\p^*-\p_k} - \Phi(\p_{k+1})\right)}^{\defeq A}
      \quad - \\
                                 &\quad \underbrace{\frac{1}{\delta}
                                 \DP{\grad\Phi(\p_{k+1})}{\p^*-\p_{k+1}}}_{\defeq
                                 B} \quad + \quad
                                 \underbrace{e^{\lambda\varphi(\p_k)}\left(
                                 f(\p_{k+1}) - f(\p^*) \right)}_{\defeq C}\\
                                 A &= \frac{1}{\delta}\left(\Phi(\p_k)
                                 + \DP{\grad\Phi(\p_k)}{\p^*-\p_k + \p_{k+1}
                               - \p_{k+1}} - \Phi(\p_{k+1})\right)\\
                                   &= \frac{1}{\delta}\left(
                                   \DP{\grad\Phi(\p_k)}{\p^*-\p_{k+1}}
                               - \BD[\Phi]{\p_{k+1}}{\p_k} \right)\\
                                   A - B &= -\DP{\frac{\grad\Phi(\p_{k+1})
                                   - \grad\Phi(\p_k)}{\delta}}{\p^*-\p_{k+1}}
                                   - \frac{1}{\delta}\BD[\Phi]{\p_{k+1}}{\p_k}
    \end{split}
  \end{equation*}
  Rewriting $C = e^{\lambda\varphi(\p_k)}\left( f(\p_{k+1}) - f(\p_k)
  + f(\p_k) - f(\p^*) \right) $, and a similar trick for the inner product
  (first term) above, we get that
  \begin{equation*}
    \begin{split}
      \frac{E_{k+1} - E_k}{\delta} &= e^{\lambda\varphi(\p_k)}\left(
      f(\p_k) - f(\p^*) \right) - \DP{\frac{\grad\Phi(\p_{k+1})
      - \grad\Phi(\p_k)}{\delta}}{\p^*-\p_k} \ \  + \\
                                   &\quad \ e^{\lambda\varphi(\p_k)}
                                   \left(f(\p_{k+1}) - f(\p_k) \right)
                                 - \DP{\frac{\grad\Phi(\p_{k+1})
                                 -  \grad\Phi(\p_k)}{\delta}}{\p_k - \p_{k+1}}
                                 - \frac{1}{\delta}\BD[\Phi]{\p_{k+1}}{\p_k}\\
                                   &= -e^{\lambda\varphi(\p_k)}\BD[f]{\p^*}{\p_k}
                                   + \underbrace{e^{\lambda\varphi(\p_k)}
                                   \BD[f]{\p_{k+1}}{\p_k} -
                                   \frac{1}{\delta}
                                 \BD[\Phi]{\p_{k+1}}{\p_k}}_{\defeq
                               \varepsilon_k^1}\\
                                   &\le -e^{\lambda\varphi(\p_k)}
                               \BD[f]{\p^*}{\p_k} \le 0.
    \end{split}
  \end{equation*}
  where the last inequality follows by assuming \emph{conformal}
  $L$-smoothness. Specifically, $\varepsilon_k^1 \le 0$ if $f$ is conformally
  $L$-smooth \wrt{} the $\lambda$-mirror flow generator $\varphi$.
\end{proof}
Using this Lyapunov potential, we can now prove the discrete analogues of
Theorem~\ref{thm:L.lambda.conv.bound} and Corollary~\ref{cor:convergence}.
\begin{theorem}
  Given the sequence $\{\p_i\}_{i=0}^{k}$ generated using the \acrshort{CBD}
  iterates~\eqref{eq:feuler-tcmf}, and convex objective $f$, we have
  \begin{equation}\label{eq:discrete_bound}
    f(\widehat{\p}_k) - f(\p^*) \le \frac{E_1}{\delta\sum_{s=1}^{k}
    e^{\lambda\varphi(\p_{s-1})}}\quad \forall \ k\ge 1
  \end{equation}
  where $E_k$ is the Lyapunov potential defined in~\eqref{eq:lyapunov_discrete},
  and $\widehat{\p_k}$ is the weighted average of the trajectory
  $\{\p_i\}_{i=1}^{k}$ defined as
  \begin{equation}
    \widehat{\p}_k \defeq \frac{\sum_{s=1}^{k} e^{\lambda\varphi(\p_{s-1})}
    f(\p_s)}{\sum_{s=1}^{k} e^{\lambda\varphi(\p_{s-1})}}.
  \end{equation}
\end{theorem}
\begin{proof}
    Define the probability distribution $p_k(x_i) \defeq
    \frac{e^{\lambda\varphi(\p_{i-1})}}{\sum_{j=1}^{k}e^{\lambda\varphi(\p_{j-1})}}$
    for $i \in \{1, \ldots, k\}$. Using this, we can define the \emph{weighted}
    average of the sequence $\p(k) \defeq (\p_i)_{i=1}^{k}$ as
    \begin{equation*}
      \widehat{\p}_k \defeq \Esubarg{p_k}{\p(k)}
      = \frac{\sum_{s=1}^{k}e^{\lambda\varphi(\p_{s-1})}
      f(\p_s)}{\sum_{s=1}^{k}e^{\lambda\varphi(\p_{s-1})}}.
    \end{equation*}
    Using Jensen's inequality on the convex objective $f$, it follows that
    \begin{align*}
      f(\widehat{\p}_k) = f\left( \Esubarg{p_k}{\p(k)} \right) &\le
      \Esubarg{p_k}{f(\p(k))} = \frac{\sum_{s=1}^{k}e^{\lambda\varphi(\p_{s-1})}
        f(\p_s)}{\sum_{s=1}^{k}e^{\lambda\varphi(\p_{s-1})}}\\
      \implies \delta\left( f( \widehat{\p}_k) - f(\p^*) \right)
       &\le \left( \sum_{s=1}^{k} e^{\lambda\varphi(\p_{s-1})}\right)^{-1} E_k
       \le \left( \sum_{s=1}^{k} e^{\lambda\varphi(\p_{s-1})}\right)^{-1} E_1\\
      \implies f(\widehat{\p}_k) - f(\p^*) &\le
      \frac{E_1}{\delta\sum_{s=1}^{k}e^{\lambda\varphi(\p_{s-1})}},
    \end{align*}
    where we have used that $E_k$ is a Lyapunov functional for $k\ge 1$.
\end{proof}
.

\vfill
\end{appendices}
